# Supplementary material for: Energy and momentum dependence of nuclear short-range correlations - Spectral function, exclusive scattering experiments and the contact formalism
Source: arXiv:1806.10217 ancillary file (2019-02-17)
Supplement: Supplementary file 1 [file Supplementary_Materials_v5.pdf]

# Supplemental Materials: Energy and momentum dependence of nuclear short-range correlations - Spectral function, Exclusive scattering experiments and the contact formalism

## SPECTRAL FUNCTION CALCULATIONS

In the paper we have presented the calculations of the spectral function as a function of $p_1$ for a fixed $\epsilon_1$ and vice versa, using the AV18 potential (See Figs. 2 and 3). Here, we present the complementary calculations using the N3LO(600) potential. See Figs. S1 and S2.

## $\#pp/\#pn$, $\#pp/\#p$ AND $\#pn/\#p$ RATIOS

In the paper we have presented the $\#pp/\#p$ ratio for $^{12}$C using the AV18 potential. Here, we present the results using the N3LO(600) potential. Fig. S3 shows the $^{12}$C $\#pp/\#p$ ratio, using the $^{12}$C contact values of the N3LO(600) potential fitted in this work.

We also present here the $\#pp/\#pn$ ratio for $^{12}$C using the AV18 and N3LO(600) potentials, see Figs. S4 and S5. The $\#pp/\#p$ ratio for $^{4}$He using the AV18 and N3LO(600) potentials is presented in Figs. S6 and S7. The $\#pn/\#p$ ratio for $^{4}$He and $^{12}$C using the AV18 and N3LO(600) potentials is presented in Figs. S8, S9, S10 and S11.

## CALCULATIONS WITH A LOCAL CHIRAL POTENTIAL

In addition to the calculations presented here and in the paper using the AV18 and N3LO(600) potentials, we have performed similar calculations using the local N2LO chiral potential [S1, S2], with cutoffs $R = 1.0$ fm and $R = 1.2$ fm, denoted here by N2LO(1.0) and N2LO(1.2). The universal two-body functions of these potentials are presented in Figs. S12 and S13. The fitted contact values for these two potentials are presented in table SI. The results for the ratios $\#pp/\#pn$, $\#pp/\#p$ and $\#pn/\#p$ are presented in Figs. S14, S15, S16 for $^{4}$He and $R = 1.0$ fm, in Figs. S17, S18, S19 for $^{4}$He and $R = 1.2$ fm, in Figs. S20, S21, S22 for $^{12}$C and $R = 1.0$ fm, and in Figs. S23, S24, S25 for $^{12}$C and $R = 1.2$ fm.

| A | potential | (e,e'pN) |
|---|---|---|
| $^{4}$He | N2LO(1.0) | $19 \pm 5$ |
| | N2LO(1.2) | $15 \pm 4$ |
| $^{12}$C | N2LO(1.0) | $19 \pm 4$ |
| | N2LO(1.2) | $20 \pm 5$ |

TABLE SI. The fitted values of the contact ratio $C^1_{pn}/C^0$ for $^{4}$He and $^{12}$C using the local chiral N2LO interaction with cutoffs $R = 1.0$ fm and $R = 1.2$ fm. The rows correspond to the different potentials and the $(e, e'pN)$ column is the fit to the experimental $\#pp/\#pn$ ratio of Ref. [S3] for $^{4}$He, and to $\#pp/\#p$ of Ref. [S4] for $^{12}$C.

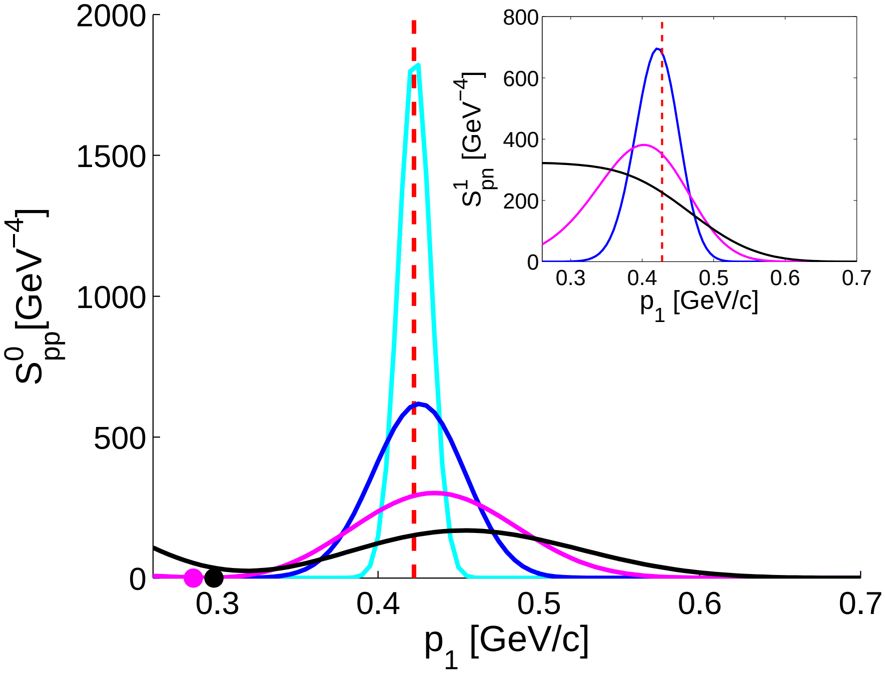


FIG. S1. $S^0_{pp}$ of $^4$He as a function of $p_1$ for fixed $\epsilon_1 = 0.82$ GeV/c, using the N3LO(600) potential and different values of $\sigma_{CM}$: 10 MeV (cyan), 30 MeV (blue), 60 MeV (magenta) and 100 MeV (black). The dashed red line is the back-to-back prediction, and the black and magenta points are the estimated location of the minimum of $S^0_{pp}$. Inset: the results for $S^1_{pn}$ for $\sigma_{CM} = 30$, 60 and 100 MeV. See the main paper for more details.

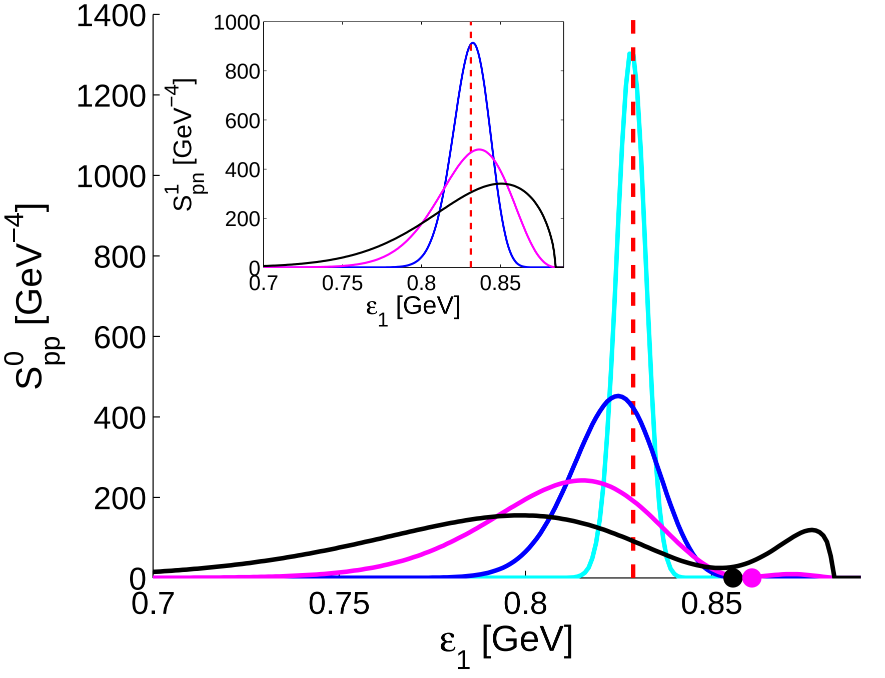


FIG. S2. The same as in Fig. S1, but as a function of $\epsilon_1$ for fixed $p_1 = 400$ MeV/c. See the main paper for more details.

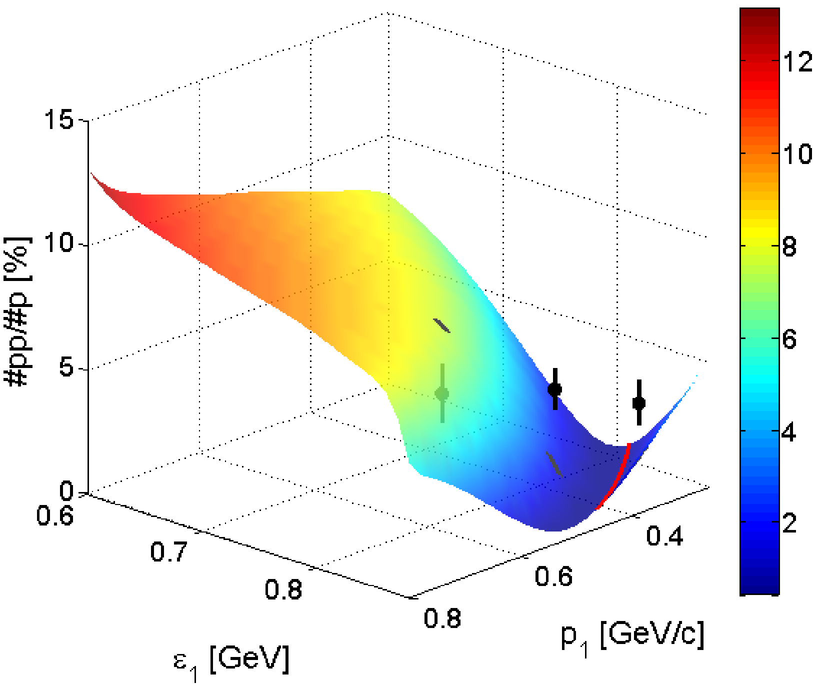


FIG. S3. The [12]C $\#pp/\#p$ ratio as a function of both $p_1$ and $\epsilon_1$, using the N3LO(600) potential. The red line is the analytic prediction for a minimal ratio value, and the black points are the experimental data of Shneor *et al.*

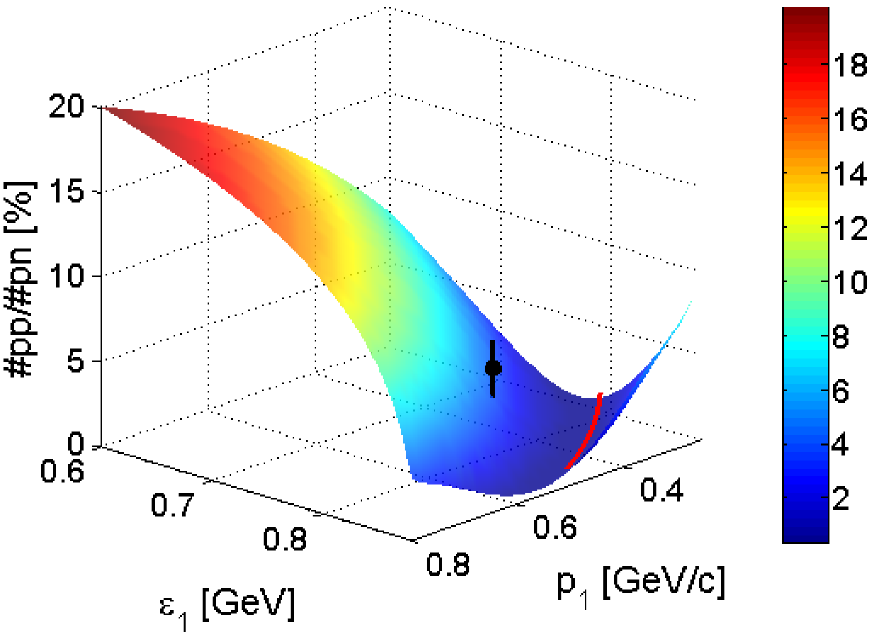


FIG. S4. The [12]C $\#pp/\#pn$ ratio as a function of both $p_1$ and $\epsilon_1$, using the AV18 potential. The red line is the analytic prediction for a minimal ratio value, and the black points are the experimental data of Subedi *et al.*

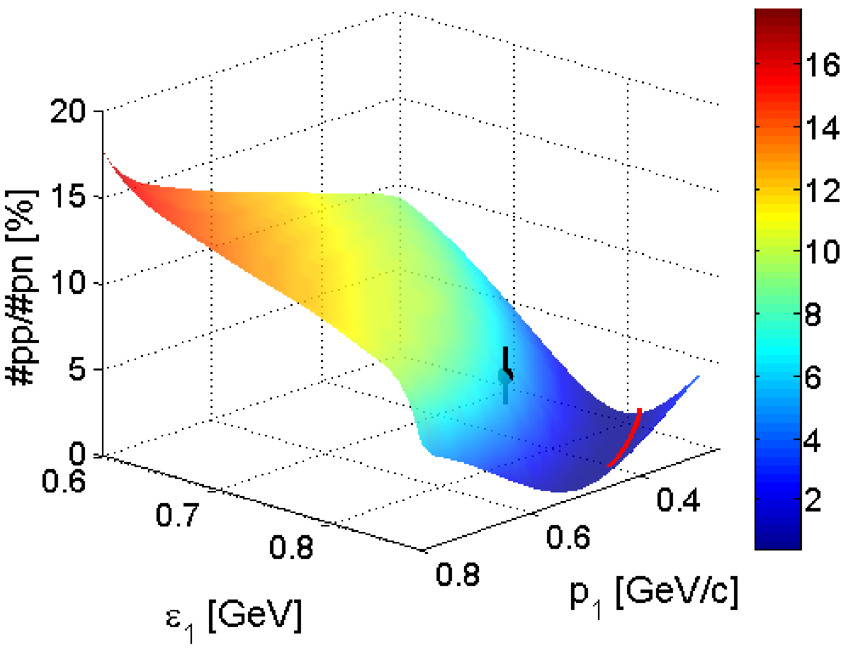


FIG. S5. The $^{12}$C $\#pp/\#pn$ ratio as a function of both $p_1$ and $\epsilon_1$, using the N3LO(600) potential. The red line is the analytic prediction for a minimal ratio value, and the black points are the experimental data of Subedi *et al.*

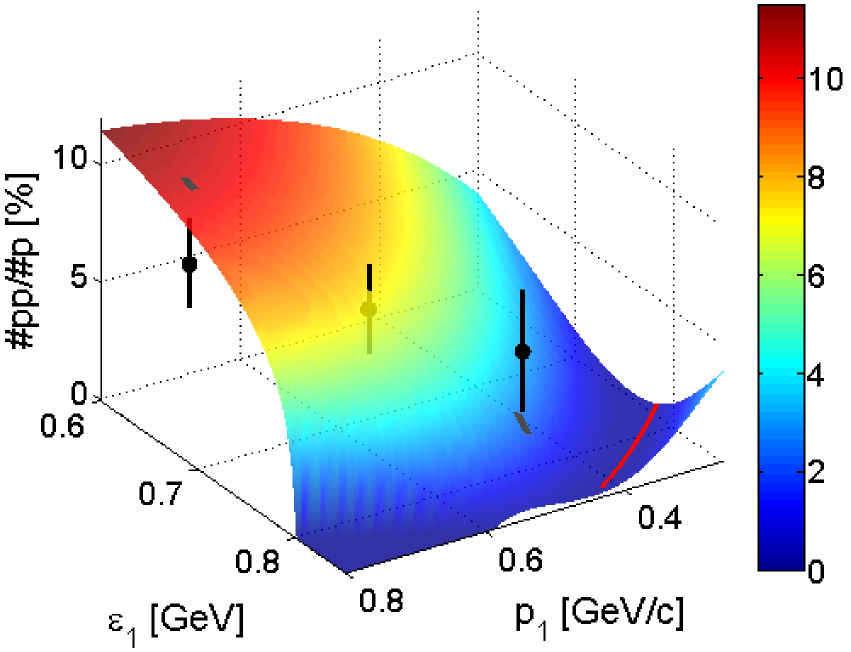


FIG. S6. The $^{4}$He $\#pp/\#p$ ratio as a function of both $p_1$ and $\epsilon_1$, using the AV18 potential. The red line is the analytic prediction for a minimal ratio value, and the black points are the experimental data of Korover *et al.*

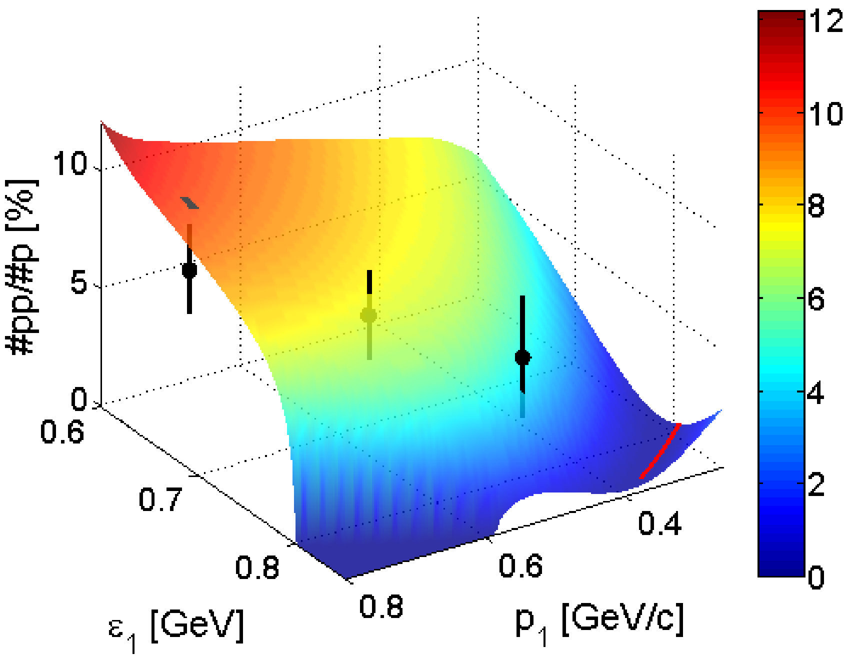


FIG. S7. The $^4$He $\#pp/\#p$ ratio as a function of both $p_1$ and $\epsilon_1$, using the N3LO(600) potential. The red line is the analytic prediction for a minimal ratio value, and the black points are the experimental data of Korover *et al.*

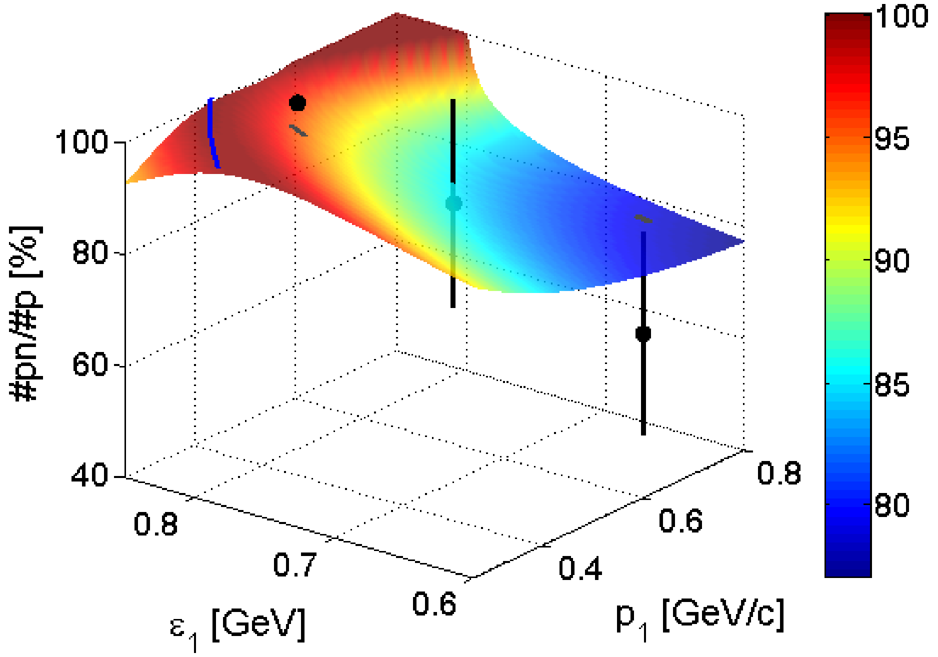


FIG. S8. The $^4$He $\#pn/\#p$ ratio as a function of both $p_1$ and $\epsilon_1$, using the AV18 potential. The blue line is the analytic prediction for a maximal ratio value, and the black points are the experimental data of Korover *et al.*

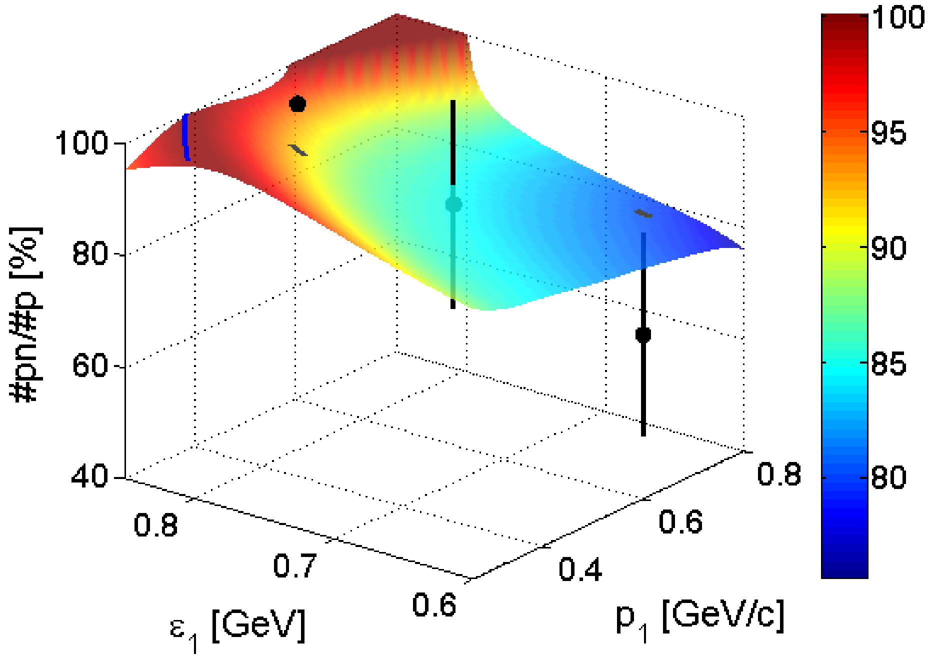


FIG. S9. The [4]He $\#pn/\#p$ ratio as a function of both $p_1$ and $\epsilon_1$, using the N3LO(600) potential. The blue line is the analytic prediction for a maximal ratio value, and the black points are the experimental data of Korover *et al.*

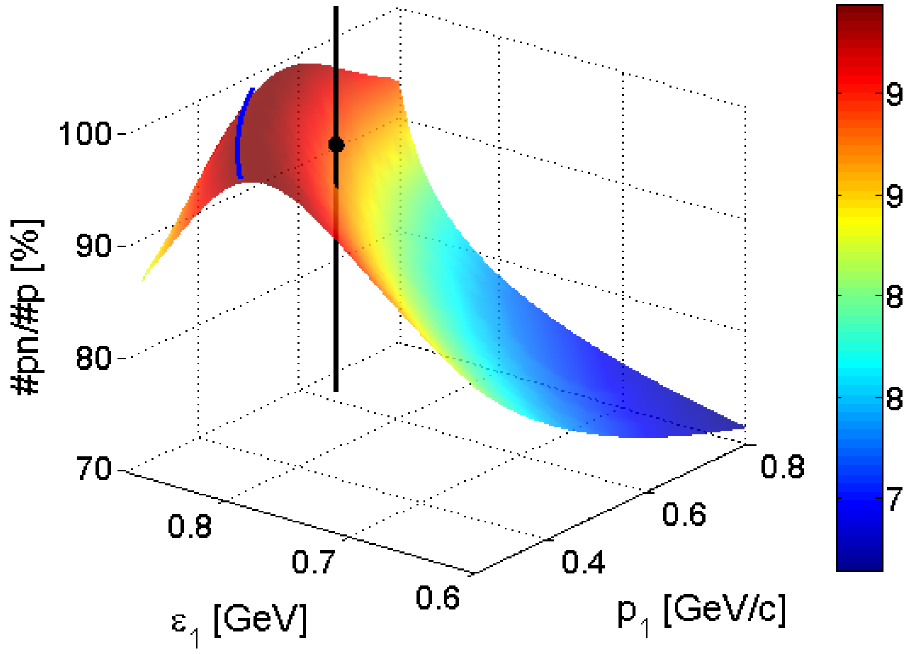


FIG. S10. The [12]C $\#pn/\#p$ ratio as a function of both $p_1$ and $\epsilon_1$, using the AV18 potential. The blue line is the analytic prediction for a maximal ratio value, and the black points are the experimental data of Subedi *et al.*

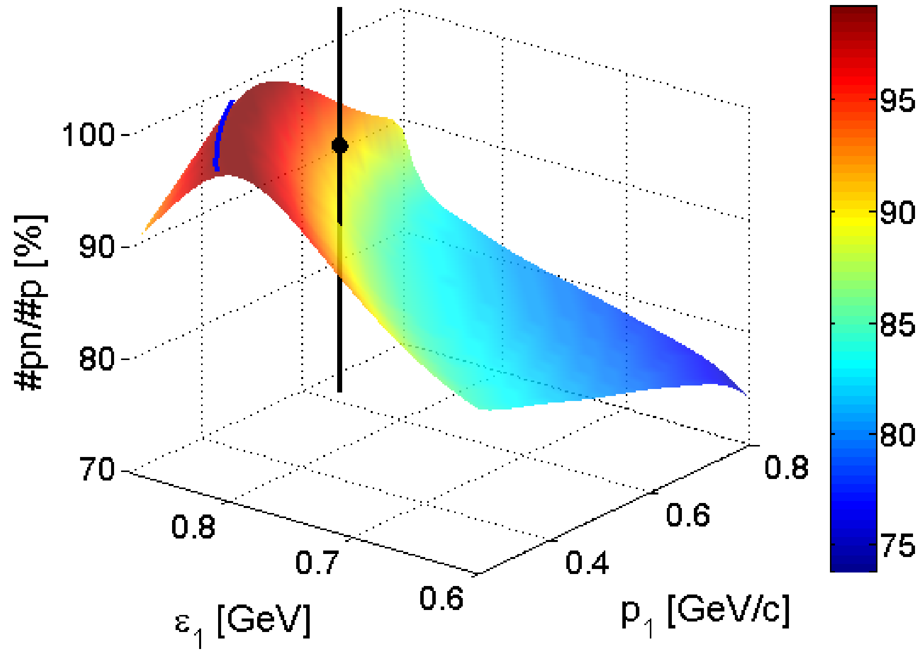


FIG. S11. The [12]C $\#pn/\#p$ ratio as a function of both $p_1$ and $\epsilon_1$, using the N3LO(600) potential. The blue line is the analytic prediction for a maximal ratio value, and the black points are the experimental data of Subedi *et al.*

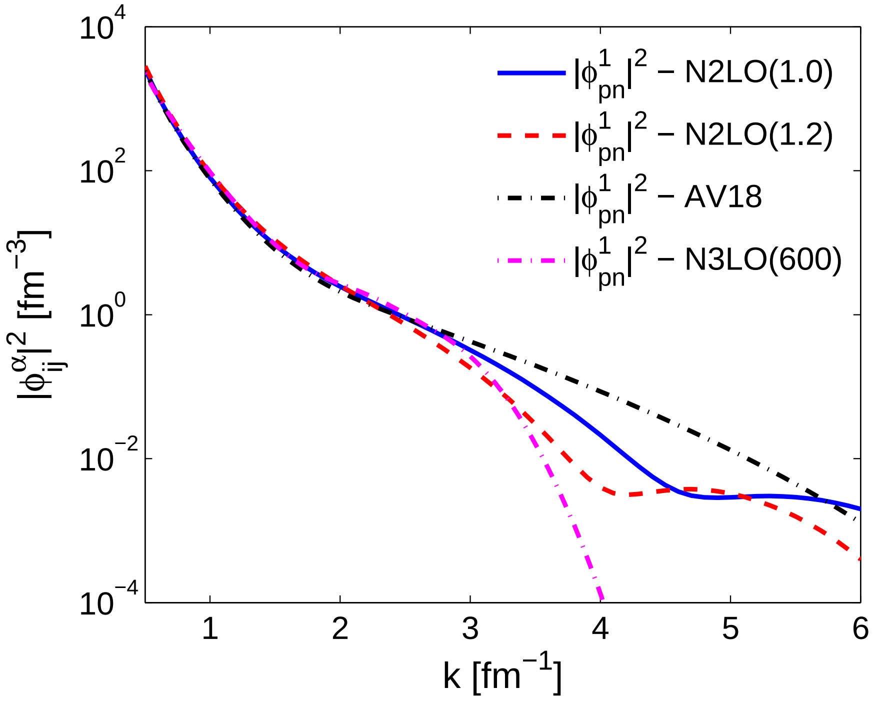


FIG. S12. The universal two-body functions for deuteron $pn$ pairs calculated using the local N2LO potentials, compared to the AV18 and N3LO(600) results. The functions are normalized such that $\int_{p_F}^{\infty} |\varphi_{ab}^{\alpha}|^2 d\boldsymbol{p}/(2\pi)^3 = 1$.

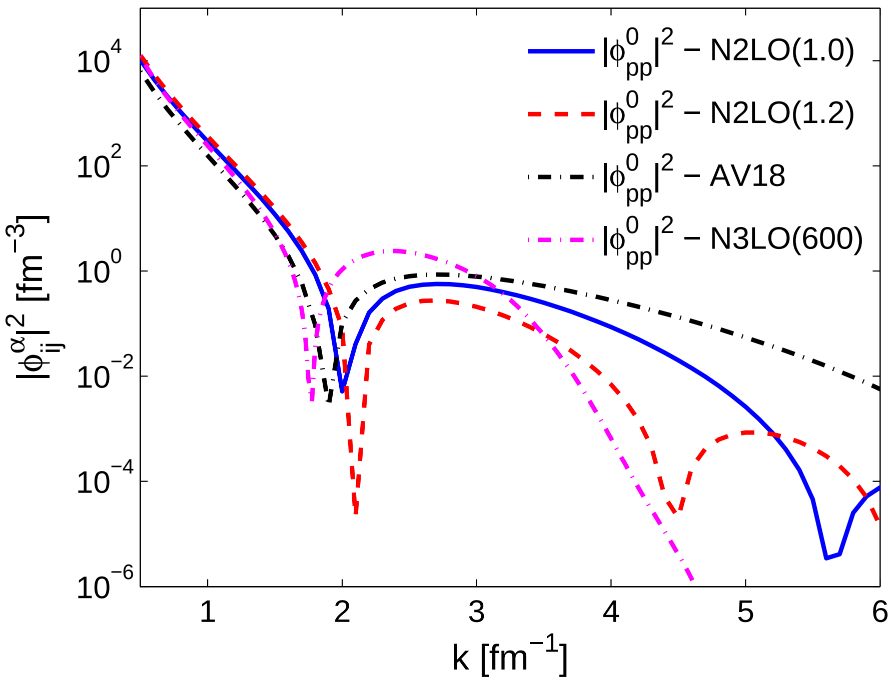


FIG. S13. The universal two-body functions for s-wave $pp$ pairs calculated using the local N2LO potentials, compared to the AV18 and N3LO(600) results. The functions are normalized such that $\int_{p_F}^{\infty} |\varphi_{ab}^{\alpha}|^2 d\boldsymbol{p}/(2\pi)^3 = 1$.

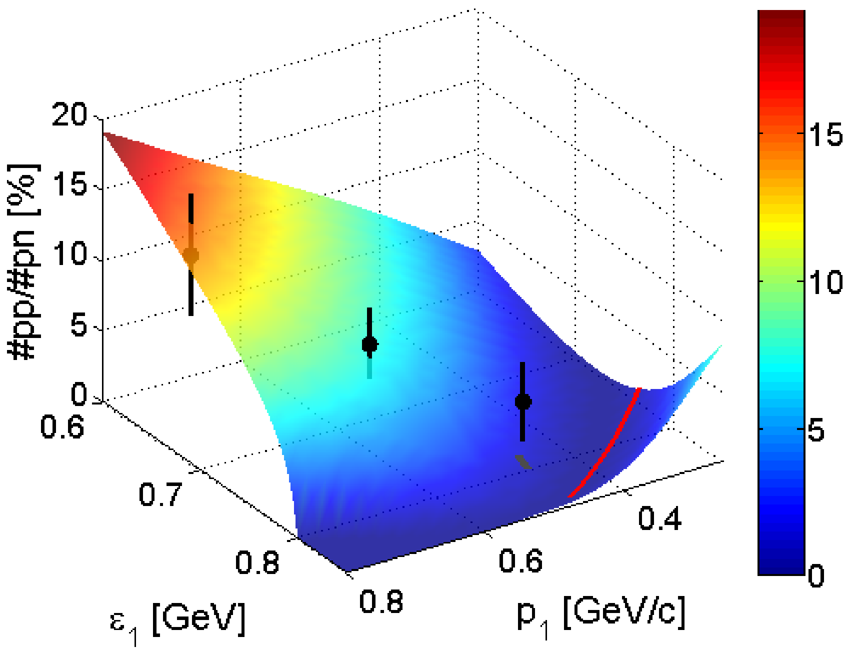


FIG. S14. The $^4$He $\#pp/\#pn$ ratio as a function of both $p_1$ and $\epsilon_1$, using the N2LO(1.0) potential. The red line is the analytic prediction for a minimal ratio value, and the black points are the experimental data of Korover *et al.*

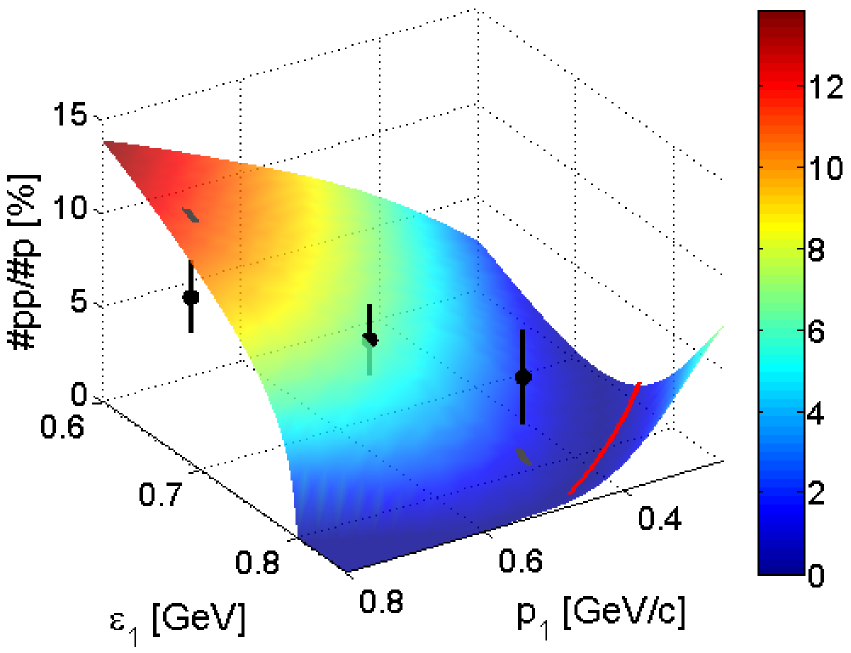


FIG. S15. The [4]He $\#pp/\#p$ ratio as a function of both $p_1$ and $\epsilon_1$, using the N2LO(1.0) potential. The red line is the analytic prediction for a minimal ratio value, and the black points are the experimental data of Korover *et al.*

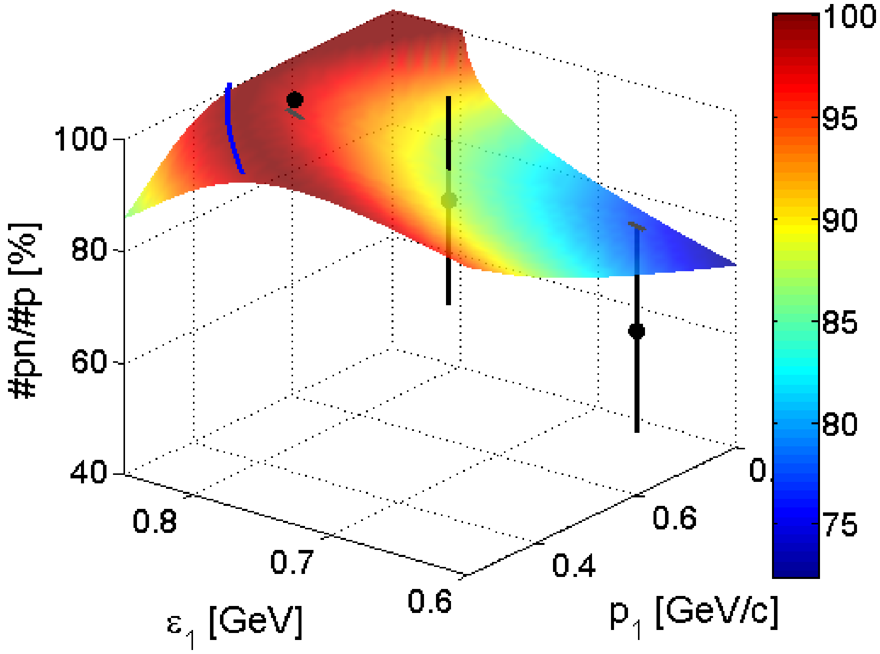


FIG. S16. The [4]He $\#pn/\#p$ ratio as a function of both $p_1$ and $\epsilon_1$, using the N2LO(1.0) potential. The blue line is the analytic prediction for a maximal ratio value, and the black points are the experimental data of Korover *et al.*

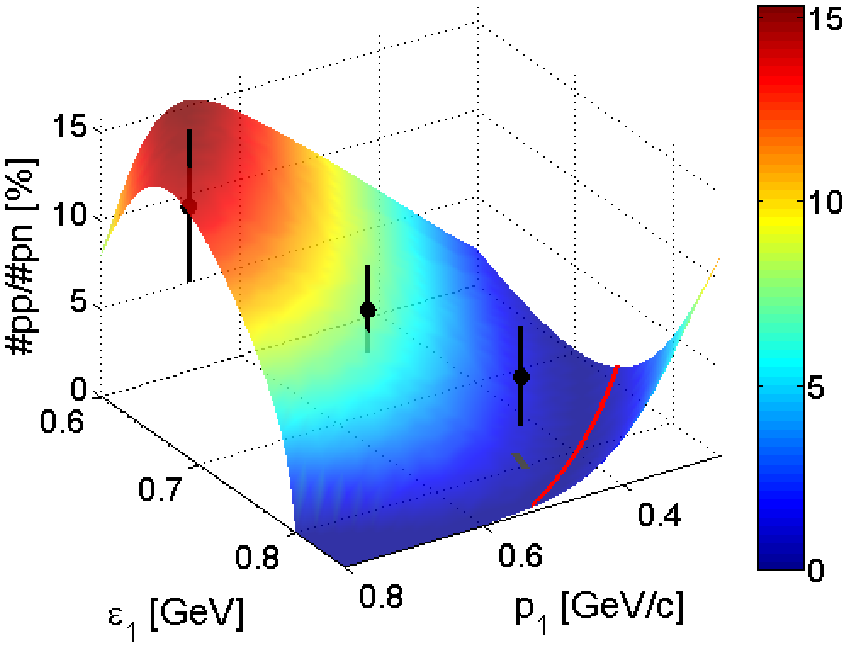


FIG. S17. The [4]He $\#pp/\#pn$ ratio as a function of both $p_1$ and $\epsilon_1$, using the N2LO(1.2) potential. The red line is the analytic prediction for a minimal ratio value, and the black points are the experimental data of Korover *et al.*

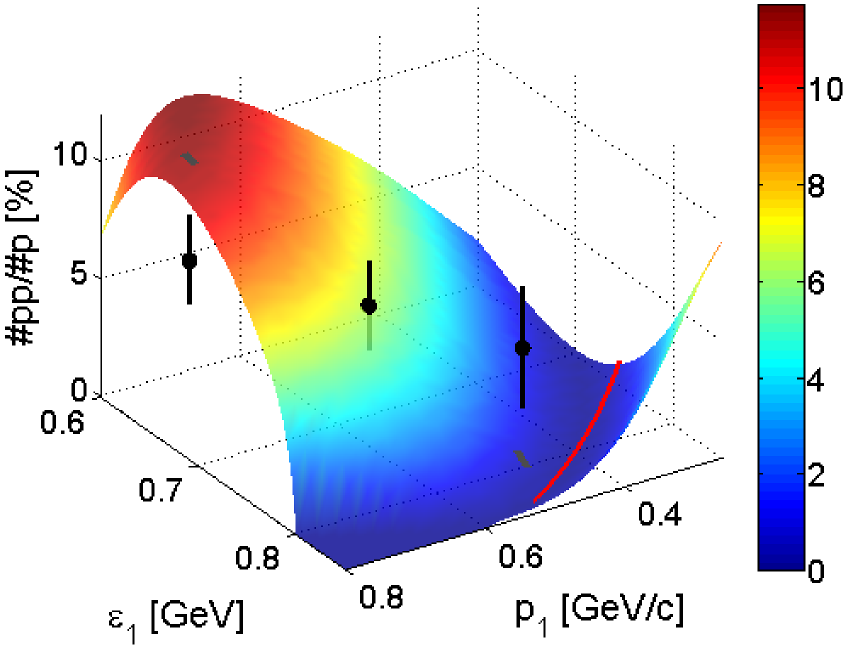


FIG. S18. The [4]He $\#pp/\#p$ ratio as a function of both $p_1$ and $\epsilon_1$, using the N2LO(1.2) potential. The red line is the analytic prediction for a minimal ratio value, and the black points are the experimental data of Korover *et al.*

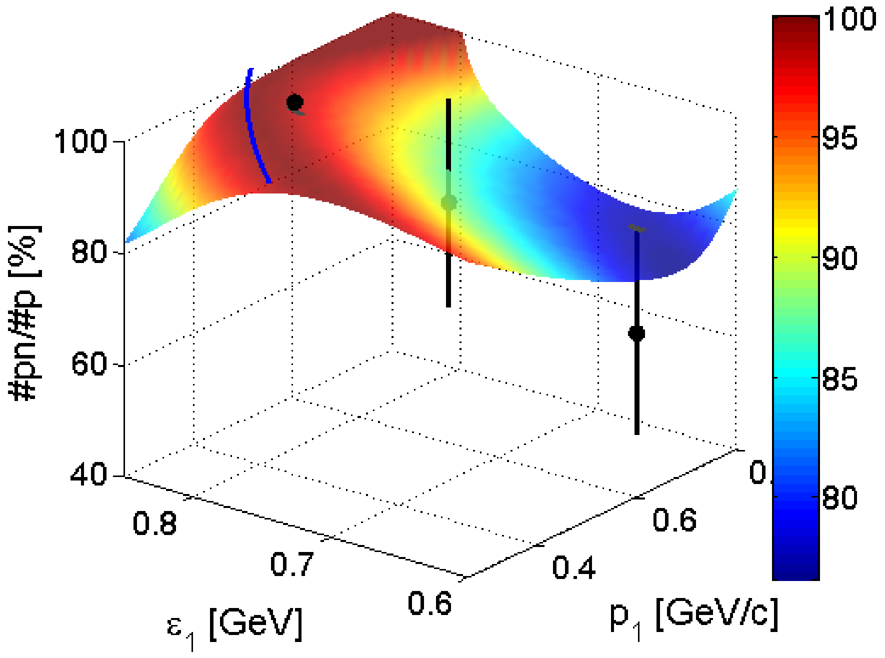


FIG. S19. The $^{4}$He $\#pn/\#p$ ratio as a function of both $p_1$ and $\epsilon_1$, using the N2LO(1.2) potential. The blue line is the analytic prediction for a maximal ratio value, and the black points are the experimental data of Korover *et al.*

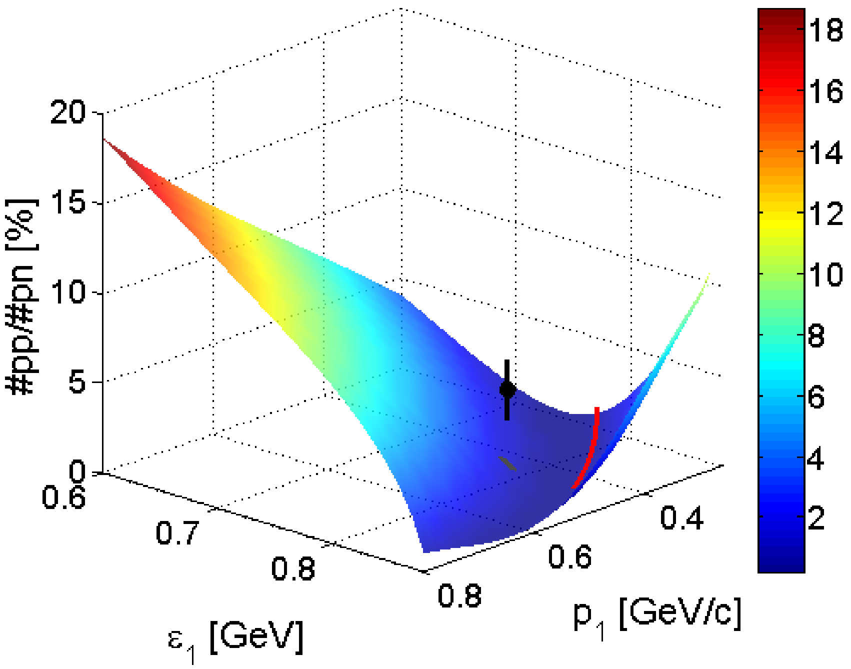


FIG. S20. The $^{12}$C $\#pp/\#pn$ ratio as a function of both $p_1$ and $\epsilon_1$, using the N2LO(1.0) potential. The red line is the analytic prediction for a minimal ratio value, and the black points are the experimental data of Subedi *et al.*

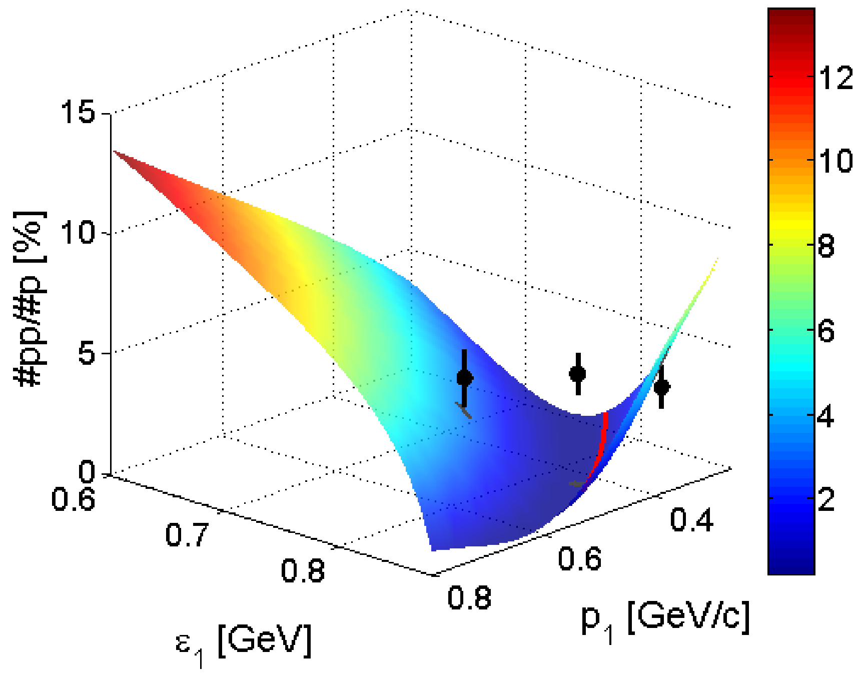


FIG. S21. The $^{12}$C $\#pp/\#p$ ratio as a function of both $p_1$ and $\epsilon_1$, using the N2LO(1.0) potential. The red line is the analytic prediction for a minimal ratio value, and the black points are the experimental data of Shneor *et al.*

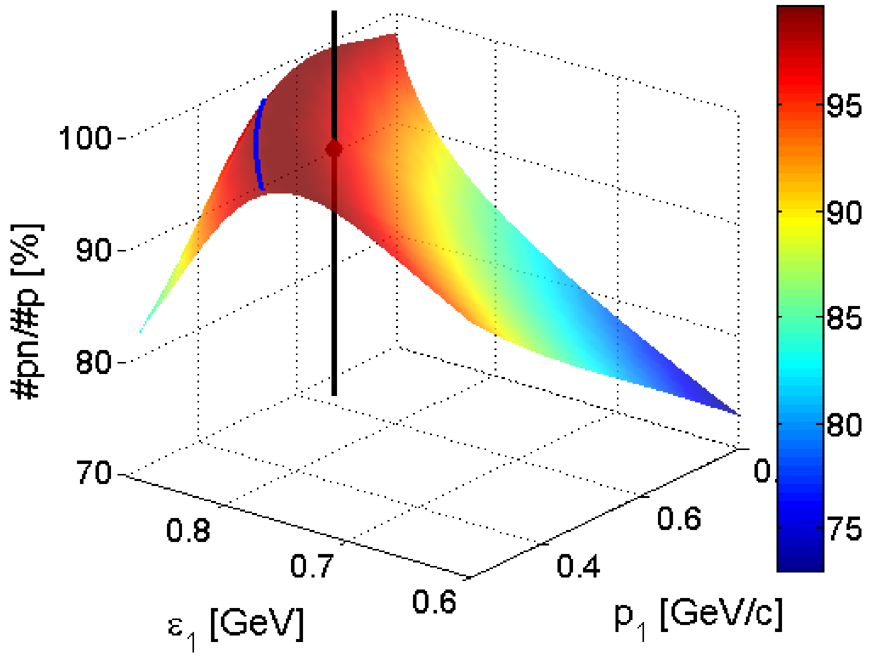


FIG. S22. The $^{12}$C $\#pn/\#p$ ratio as a function of both $p_1$ and $\epsilon_1$, using the N2LO(1.0) potential. The blue line is the analytic prediction for a maximal ratio value, and the black points are the experimental data of Subedi *et al.*

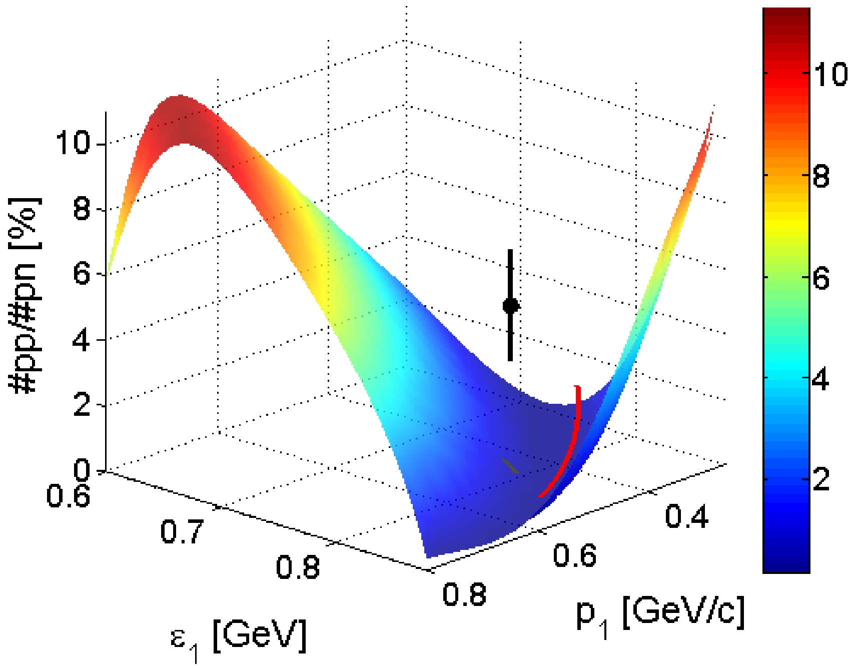


FIG. S23. The [12]C $\#pp/\#pn$ ratio as a function of both $p_1$ and $\epsilon_1$, using the N2LO(1.2) potential. The red line is the analytic prediction for a minimal ratio value, and the black points are the experimental data of Subedi *et al.*

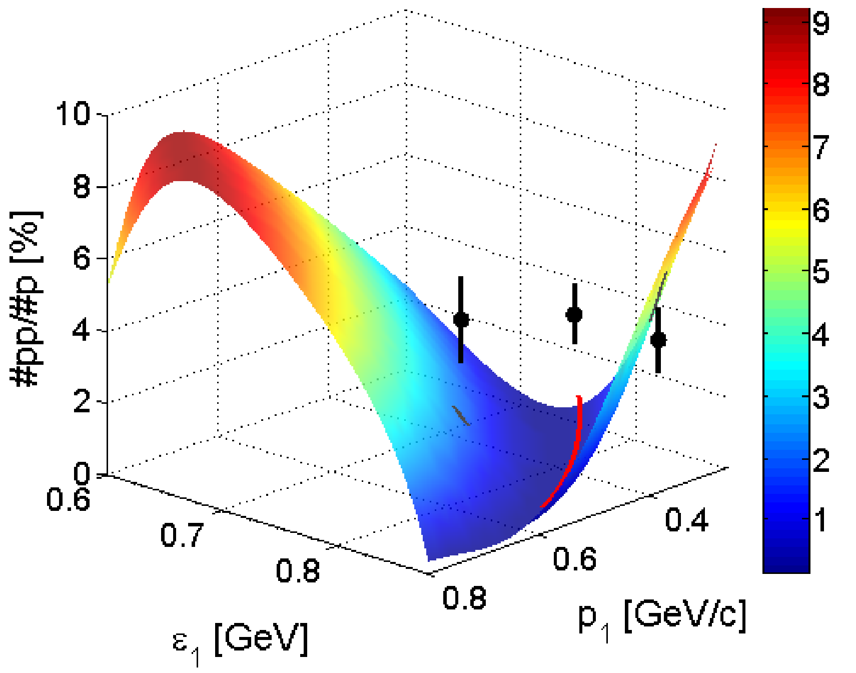


FIG. S24. The [12]C $\#pp/\#p$ ratio as a function of both $p_1$ and $\epsilon_1$, using the N2LO(1.2) potential. The red line is the analytic prediction for a minimal ratio value, and the black points are the experimental data of Shneor *et al.*

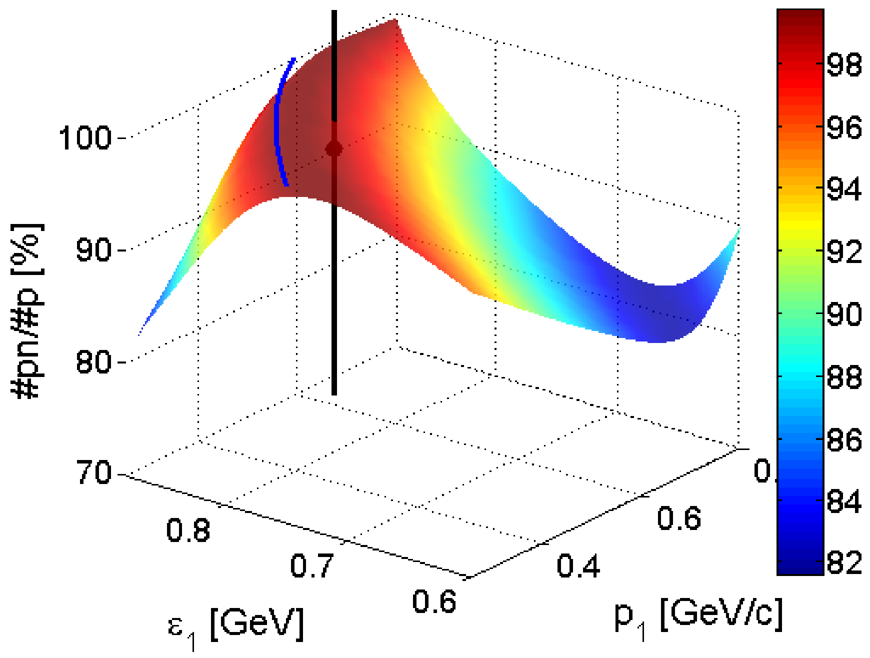


FIG. S25. The $^{12}$C $\#pn/\#p$ ratio as a function of both $p_1$ and $\epsilon_1$, using the N2LO(1.2) potential. The blue line is the analytic prediction for a maximal ratio value, and the black points are the experimental data of Subedi *et al.*

## COMPARISON WITH THE CONVOLUTION MODEL

As mentioned in the paper, our model for the spectral function is similar to the convolution model [S5–S8]. The convolution model spectral function is given by

$$S^p(\boldsymbol{k}_1, E) = \int n_{rel}^{pn}\left(\left|\boldsymbol{k}_1 - \frac{\boldsymbol{K}_{CM}}{2}\right|\right) n_{CM}^{pn}(\boldsymbol{K}_{CM})\delta\left(E - E_{thr}^p - \frac{A-2}{2m(A-1)}\left[\boldsymbol{k}_1 - \frac{(A-1)\boldsymbol{K}_{CM}}{A-2}\right]^2\right) d^3K_{CM}$$
$$+2\int n_{rel}^{pp}\left(\left|\boldsymbol{k}_1 - \frac{\boldsymbol{K}_{CM}}{2}\right|\right) n_{CM}^{pp}(\boldsymbol{K}_{CM})\delta\left(E - E_{thr}^p - \frac{A-2}{2m(A-1)}\left[\boldsymbol{k}_1 - \frac{(A-1)\boldsymbol{K}_{CM}}{A-2}\right]^2\right) d^3K_{CM} \quad \text{(S1)}$$

where

$$E_{thr}^p = |E_A| - |E_{A-1}|, \quad \text{(S2)}$$

$E_A$ and $E_{A-1}$ are the ground state energies, and

$$E^* = E - E_{thr}. \quad \text{(S3)}$$

The $pn$ relative momentum distribution is given by

$$n_{rel}^{pn}(k_{rel}) = C_A^{pn} n_D(k_{rel}), \quad \text{(S4)}$$

where $n_D(k_{rel})$ is the deuteron momentum distribution and $C_A^{pn}$ is the appropriate contact. For $pp$ pairs

$$n_{rel}^{pp}(k_{rel}) = \frac{n^{pp}(k_{rel}, K_{CM} = 0)}{n_{CM}(K_{CM} = 0)}, \quad \text{(S5)}$$

where $n^{pp}(k_{rel}, K_{CM})$ is the two-body $pp$ momentum distribution.

In both this model and ours, the asymptotic high-momentum spectral function is calculated as a convolution of the relative momentum distribution with the CM distribution, constrained by the energy-conserving delta function. Nevertheless, there are few differences between the two models:

1. *pn* channels - In our model we consider two *pn* functions, while in the convolution model only the deuteron channel is used. The deuteron channel is expected to be the dominant one.

2. Integration domain - Since the factorization of the total wave function holds only for high relative momentum, there is a need to introduce a cutoff to the integrals in the two models. In our calculations we use the sharp restriction $k_{rel} > k_F$, while in the recent convolution model papers the restriction $k_{rel} > 1.0\ \text{fm}^{-1} + 0.5K_{CM}$ is used.

3. CM distribution - We use the experimental Gaussian CM distribution, while in the recent convolution model papers an ab-initio CM distribution is used.

4. Relativistic expressions and energy definition - We use relativistic expression for the energy of the spectator nucleon $\epsilon_2$ while in the convolution model non-relativistic expressions are used. Additionally, in the energy conservation of the convolution model only the internal energy of the (A-1) system is considered, while we include also the CM energy. This means that our definition of $\epsilon_1$ is different than the convolution model definition of $E$.

The differences in the definitions of the energy, discussed in point 4, complicate the comparison between the two models. For the purpose of this comparison, we will use the energy definition of the convolution model also in our calculations, i.e. we will use the delta function appearing in Eq (S1). This will allow us to study the effects of the differences mentioned in points 1-3 on the resulting spectral function. We will compare here our calculations to the results appearing in Fig. 11 of Ref. [S8], where the spectral function was calculated using the convolution model, for $p_1 = 3.5\ \text{fm}^{-1}$ as a function of $E^*$, for different nuclei.

In fig. S26 we present the *pn* contribution to the spectral function of $^4$He using the two models. Both the spin-one (deuteron) and spin-zero contributions of the contact formalism are shown, calculated with $\sigma_{CM} = 100$ MeV. The contact values are taken from the momentum-space results of Ref. [S9]. The convolution model includes only a single *pn* contribution as discussed above. According to Ref. [S10] (table I), the $^4$He deuteron contact extracted from the VMC data of Ref. [S11], used in the contact calculations, is larger by a factor of 5/4 than the value used in the convolution model calculations. Therefore, in order to compare the two models, the convolution model results should be multiplied by a factor of 5/4. Taking this correction into account, a nice agreement is observed between the convolution model results and the deuteron-channel contribution of the contact calculations. This means that the differences discussed in points 2 and 3 above have only a small effect on the final spectral function. Regarding point 1, notice that the spin-zero contribution is of the order of 10% of the spin-one contribution, i.e. it is a sub-leading but sizable term, that is not taken into account in the convolution model.

Similar results are presented in Fig. S27 for $^{12}$C, using $\sigma_{CM} = 143$ MeV in the contact calculations. For $^{12}$C, according to Refs. [S9] and [S10], similar values of the deuteron contacts were used in the two models (after taking into account the different normalization conventions of the deuteron two-body function), and therefore we would expect an agreement between the contact and convolution models without any need for corrections. Nevertheless, it is clear from Fig. S27 that only after multiplying the convolution model results by a factor of about 1.35, a good agreement is observed between the deuteron contribution of the two models. It is possible that for $^{12}$C the differences discussed in points 2 and 3 become more significant, although the similar energy dependence of the two models might indicate a different origin for this disagreement, which is not understood at this point.

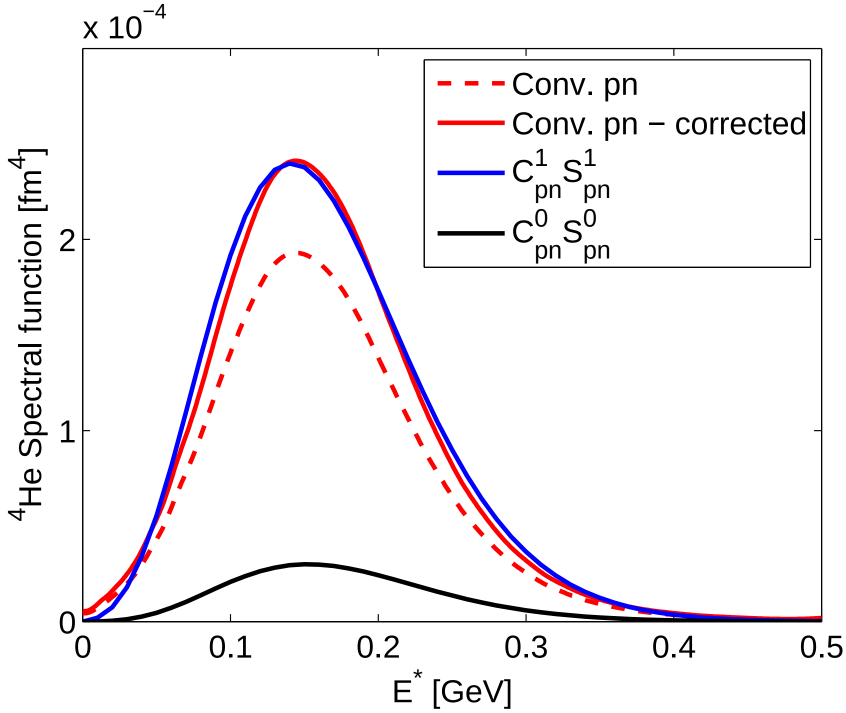


FIG. S26. The $pn$ contribution to the $^4$He $S^p(p_1, E^*)$ for $p_1 = 3.5$ fm$^{-1}$ as a function of $E^*$. The blue and black lines are the deuteron (spin-one) and spin-zero contributions of the contact formalism, respectively, adapted to the non-relativistic energy definition of the convolution model. The dashed red line is the $pn$ contribution of the convolution model, taken from Fig. 11 of Ref. [S8]. The solid red line is the same as the dashed line, but multiplied by 5/4, to correct for the different contact values used in the two models.

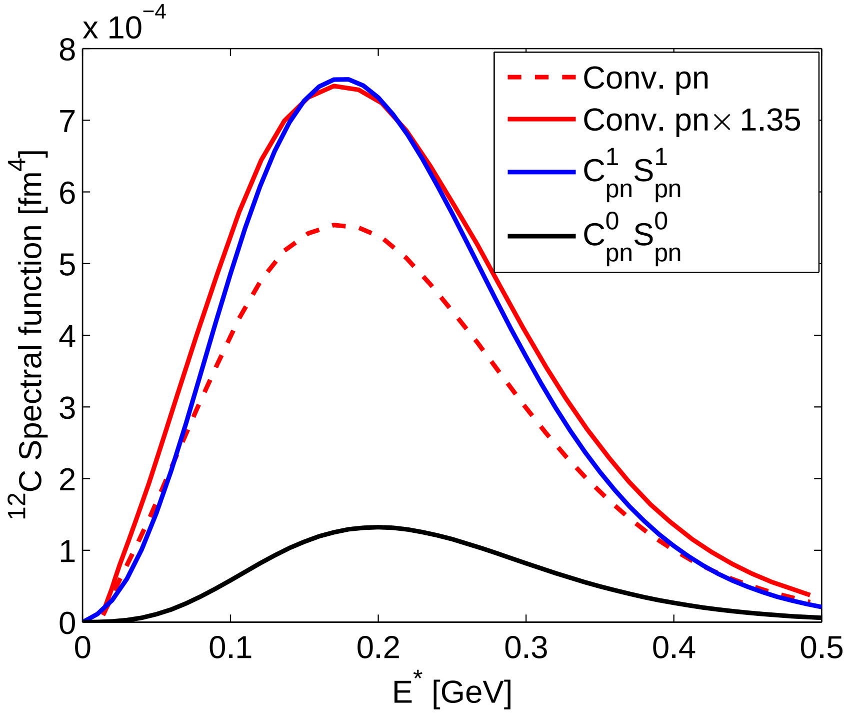


FIG. S27. The same as in Fig. S26 but for $^{12}$C. The solid red line is the same as the dashed line, but multiplied by 1.35.

[S1] A. Gezerlis, I. Tews, E. Epelbaum, S. Gandolfi, K. Hebeler, A. Nogga, and A. Schwenk, Phys. Rev. Lett. **111**, 032501 (2013)
[S2] A. Gezerlis, I. Tews, E. Epelbaum, M. Freunek, S. Gandolfi, K. Hebeler, A. Nogga, and A. Schwenk, Phys. Rev. C **90**, 054323 (2014)
[S3] I. Korover, *et al.*, Phys.Rev.Lett. **113**, 022501 (2014).
[S4] R. Shneor, *et al.*, Phys. Rev. Lett. **99**, 072501 (2007)
[S5] C. Ciofi degli Atti, S. Simula, L. L. Frankfurt, and M. I. Strikman, Phys. Rev. C **44**, R7(R) (1991)
[S6] C. Ciofi degli Atti and S. Simula, Phys. Rev. C **53**, 1689 (1996).
[S7] C. Ciofi degli Atti, C. B. Mezzetti, and H. Morita Phys. Rev. C **95**, 044327 (2017)
[S8] C. Ciofi degli Atti and H. Morita Phys. Rev. C **96**, 064317 (2017)
[S9] R. Weiss, R. Cruz-Torres, N. Barnea, E. Piasetzky, and O. Hen, Phys. Lett. B **780**, 211 (2018)
[S10] M. Alvioli, C. Ciofi degli Atti, and H. Morita, Phys. Rev. C **94**, 044309 (2016)
[S11] R. B. Wiringa, R. Schiavilla, S. C. Pieper, J. Carlson, Phys. Rev. C **89**, 024305 (2014).
